# Supplementary material for: Crossed graphene nanoribbons as beam splitters and mirrors for electron quantum optics
Source: arXiv:2005.11391 source file (2020-07-27)
Supplement: Supplementary file 1 [file supp-material.pdf]

# Supplementary information
# Crossed graphene nanoribbons as beam splitters and mirrors for electron quantum optics

Sofia Sanz,[1,*] Pedro Brandimarte,[1] Géza Giedke,[1,2] Daniel Sánchez-Portal,[1,3] and Thomas Frederiksen[1,2,†]

[1]*Donostia International Physics Center (DIPC) – UPV/EHU, Paseo Manuel de Lardizabal 4, E-20018, Donostia-San Sebastián, Spain*
[2]*IKERBASQUE, Basque Foundation for Science, E-48011, Bilbao, Spain*
[3]*Centro de Física de Materiales (CFM) CSIC-UPV/EHU, Paseo Manuel de Lardizabal 5, E-20018, Donostia-San Sebastián, Spain*
(Dated: July 27, 2020)

## CONTENTS

S1. Electron transport as a function of the intersecting angle 2

S2. Bond currents 3

S3. Scattering potentials 5

S4. Transmission matrices 6

S5. Band structure of monolayer and bilayer GNRs 20

S6. Transmission peaks as a function of the ribbon width 21

S7. Robustness of transport properties for AA-stacked ZGNRs 22

References 27

* sofia.sanz@dipc.org
† thomas_frederiksen@ehu.eus

## S1. ELECTRON TRANSPORT AS A FUNCTION OF THE INTERSECTING ANGLE

In this section we compute the transmission and reflection probabilities, and the figure of merit (Eq. (11)) as a function of the intersecting angle between the two crossed ribbons. In Fig. S1 we show results for several intersecting angles $\theta = [30°, 90°]$ for AA- and AB-stacked crossed 8-ZGNRs. All the rotations are performed around the center of the scattering region defined for these two mentioned high-symmetry configurations existing for $\theta = 60°$.

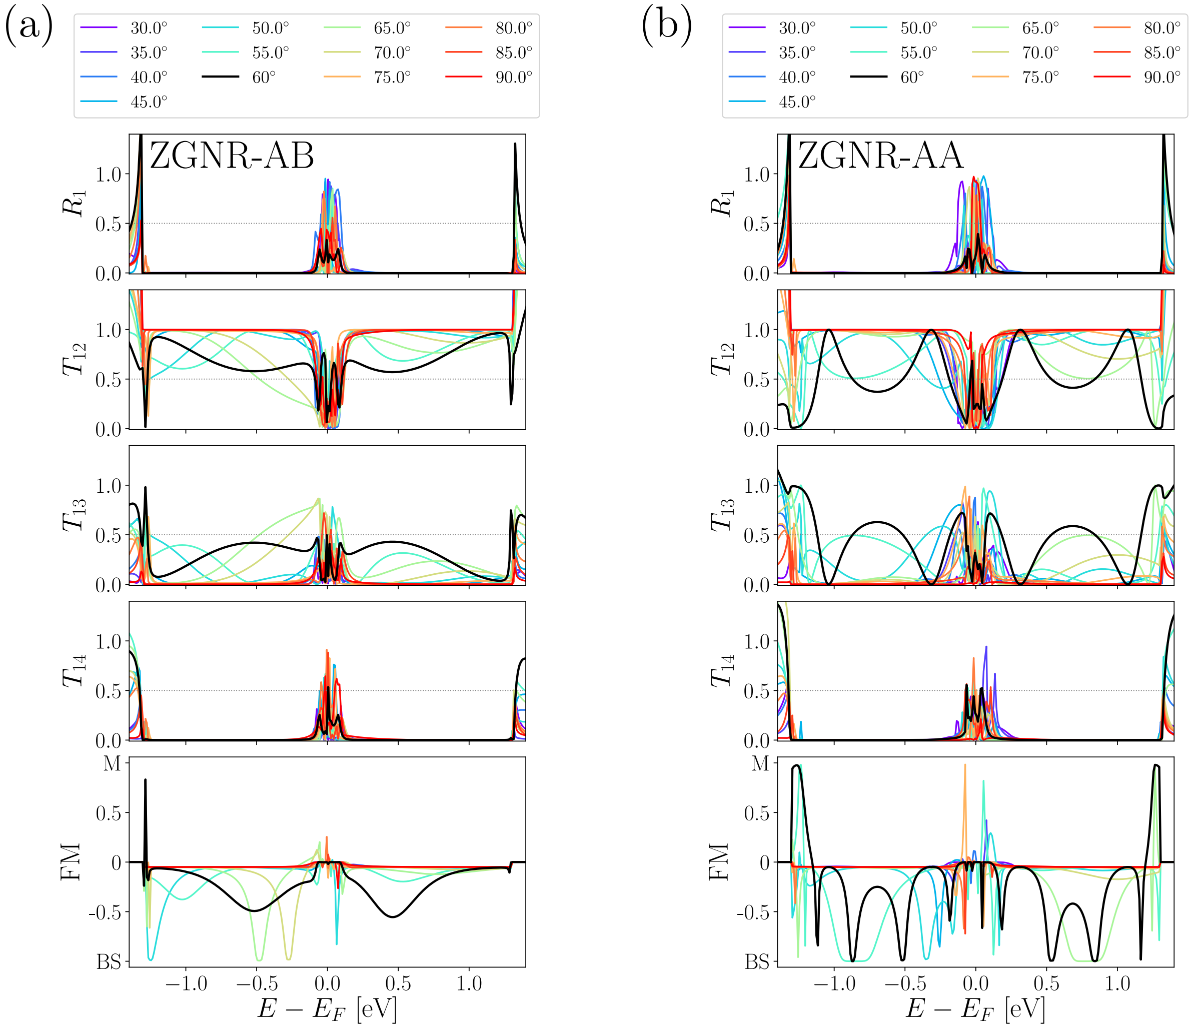


FIG. S1. Transmission probabilities as a function of the intersectin angle for crossed 8-ZGNRs. Reflection $R_1$ and transmission probabilities $T_{12}, T_{13}, T_{14}$, and figure of merit $FM$ as a function of the intersecting angle between the two ZGNRs for the (a) AB-stacked and (b) AA-stacked cases.

## S2. BOND CURRENTS

In this section we analyze the transport properties of multi-terminal devices in real space by computing the bond currents [1], defined as

$$J_{ij} = \mathrm{Im}\left[H_{ji}A_\alpha(i,j) - H_{ij}A_\alpha(j,i)\right] \tag{S1}$$

where $H_{ij}$ denotes the matrix element of the Hamiltonian of Eq. (2), and $A_\alpha(i,j)$ is the matrix element of the spectral density of scattering states [Eq. (9)] for electrons incoming from lead $\alpha = 1$, between nearest neighbor atoms $i, j$. There is an implicit energy dependency on $J_{ij}$ and $A_\alpha$.

Similar results are shown in Fig. 3, where the spectral density of the scattering states are plotted. However, the spectral density of states, defined in Eq. (9), also contains the contribution to the DOS of non-propagating (localized) states, that do not contribute to the electron transport. For this reason, we complement those results by plotting the current flowing between the different pairs of atoms, as defined in Eq. (S1), where we see the real space distribution of the propagating scattering states.

The bond currents in Fig. S2 were obtained with TBTrans [2].

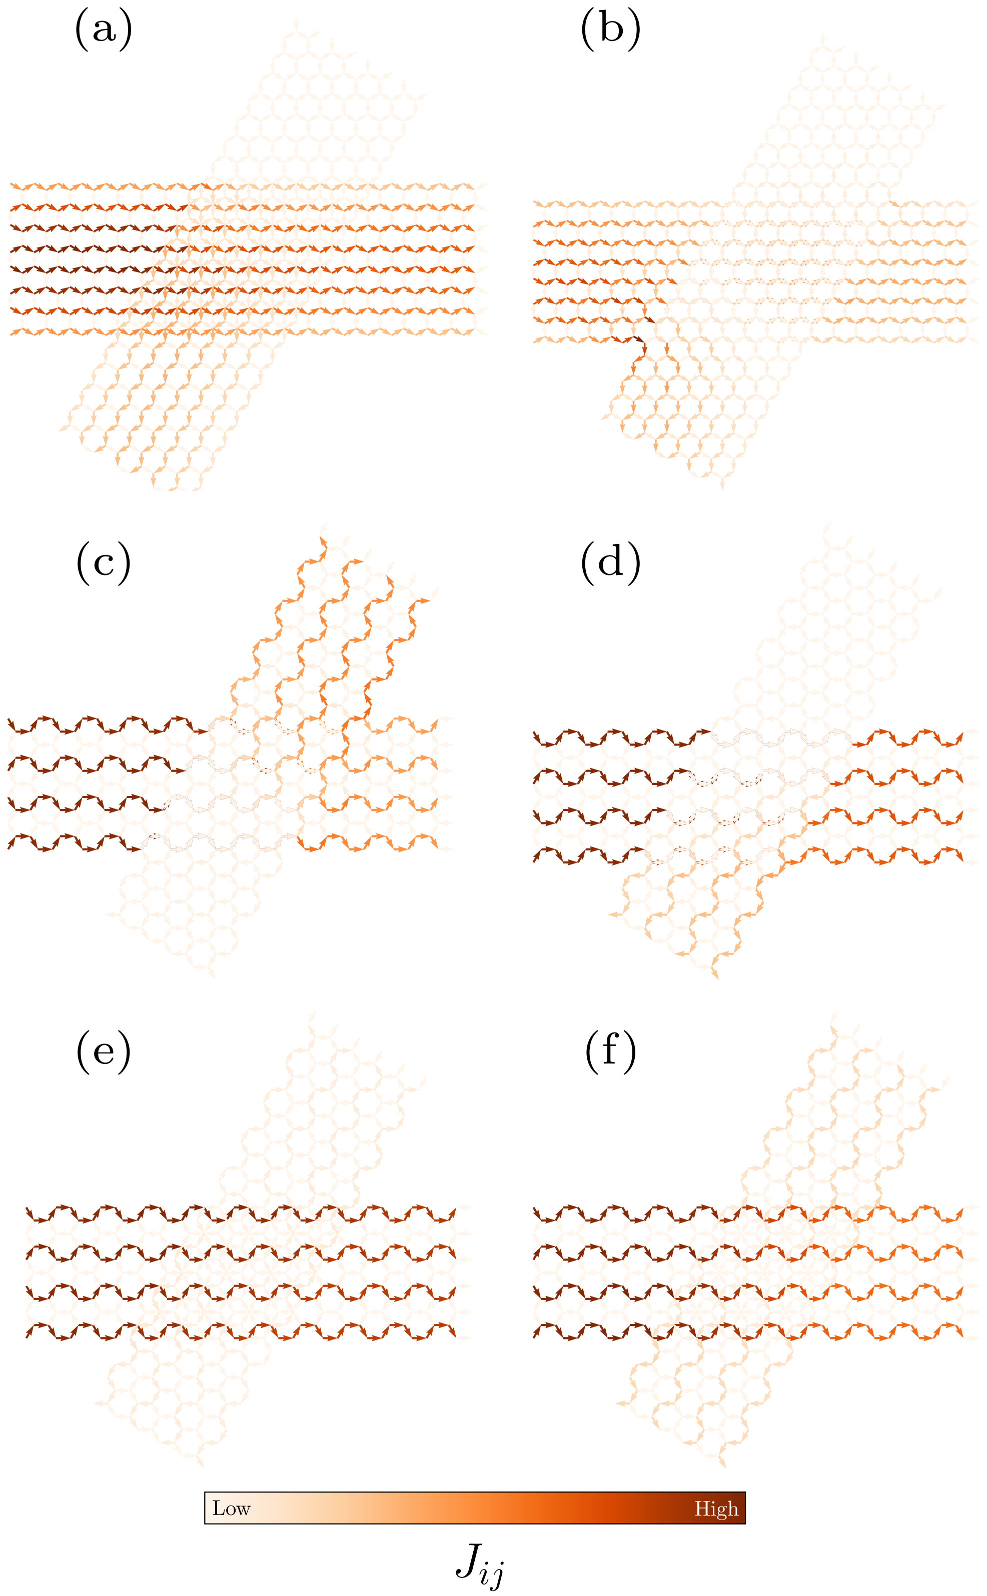


FIG. S2. Bond currents of scattering electrons incoming from electrode $\alpha = 1$ obtained from Eq. (S1), for the same geometries of the four-terminal devices as defined in Fig. 2: (a) 8-ZGNR `AB`, (b) 8-ZGNR `AA`, (c) 11-AGNR `AA-1`, (d) 11-AGNR `AA-2`, (e) 11-AGNR `AB-1`, and (f) 11-AGNR `AB-2`. The bond currents were calculated at $E = 200$ meV for ZGNR-based devices and $E = 0$ meV for AGNR-based devices. The arrows in all plots determine the direction of the bond current between atoms $i, j$.

## S3. SCATTERING POTENTIALS

In this section we analyse in more detail the scattering potentials created by the inter-GNRs coupling between the crossed ribbons for each of the devices of Fig. 2. The black dots in Fig. S3 indicate the atoms of the two ribbons that lie one on top of the other (stacked atoms), *i.e.*, that possess the same $xy$-coordinates. Similarly to Fig. 2, we show the reflection symmetry planes (red dashed lines) that leave the geometries of Fig. S3 unchanged. One thing that is worth mentioning, is that not only the geometry generated by the overlapping atoms (Fig. S3) determines the symmetry, but in principle also their local environment, especially for those located at the borders of the intersection. However, the atoms that lie one on top of the other will give the main contribution to the scattering potential, as they contribute with the strongest interatomic coupling elements. For this reason the symmetries indicated in Fig. S3 apply approximately to the full problem.

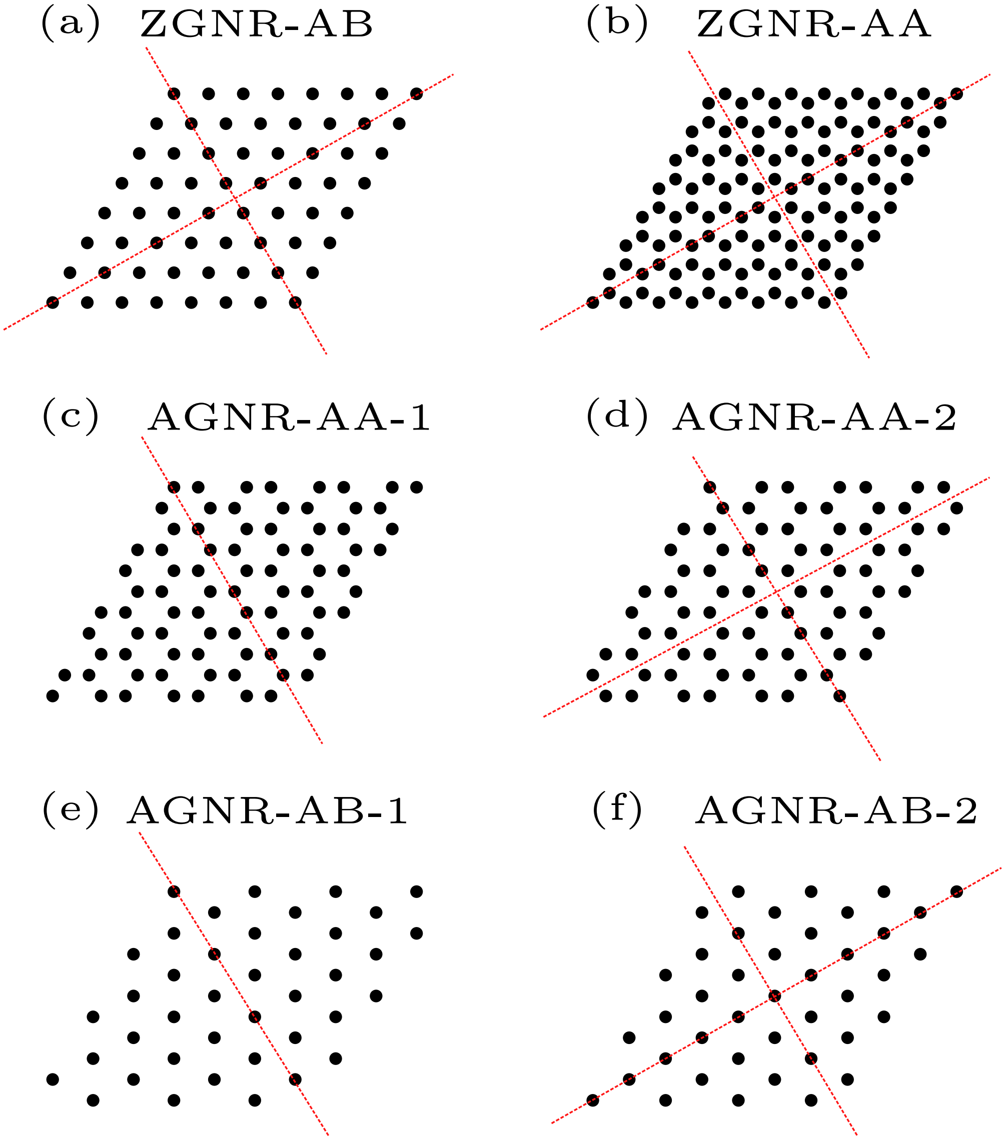


FIG. S3. Stacked atoms extracted from the crossing between two GNRs. The black dots indicate the geometry created by the atoms that lie one on top of the other in the junctions of Fig. 2: (a) 8-ZGNR-AB, (b) 8-ZGNR-AA, (c) 11-AGNR-AA-1, (d) 11-AGNR-AA-2, (e) 11-AGNR-AB-1 and (f) 11-AGNR-AB-2. The red dashed lines indicate the symmetry planes (reflection) planes that preserve the geometries described by the stacked atoms.

## S4. TRANSMISSION MATRICES

In order to complement the results presented in the main text, we compute here the transmission matrices as described in Eq. (10) for all edge terminations and stacking configurations.In the main text we showed the example of AB-stacked ZGNRs (Fig. 4). Here, Figs. S4-S16 provide the analogous results for all the other cases. In addition, there are three families according to the width of the ribbon for the cases of AGNR devices ($W = 3p$, $3p + 1$, and $3p + 2$) [3–6]. Therefore, the transmission probability matrix is plotted for each configuration (`AA-1`, `AA-2`, `AB-1` and `AB-2`) and family separately. We only show results for energies where there is only one band, *i.e.*, white regions in Figs. S4 - S14 correspond to energies where the number of bands is zero (gap) or larger than one (multiple electronic bands).

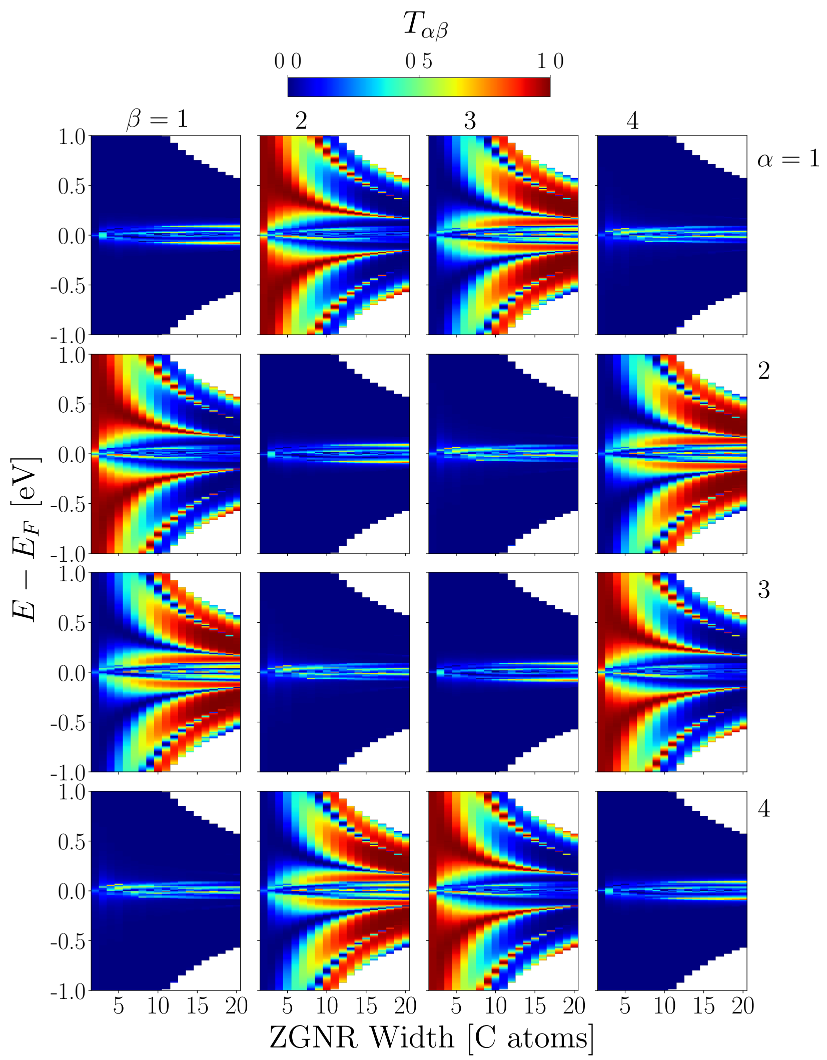


FIG. S4. Transmission probabilities $T_{\alpha\beta}$ between all the electrode pairs for ZGNR systems in the the `AA` configuration as a function of the ribbon width $W$ and electron energy $E - E_F$. The different rows mean the incoming electrode $\alpha$, while the different columns represent the outgoing electrode $\beta$.

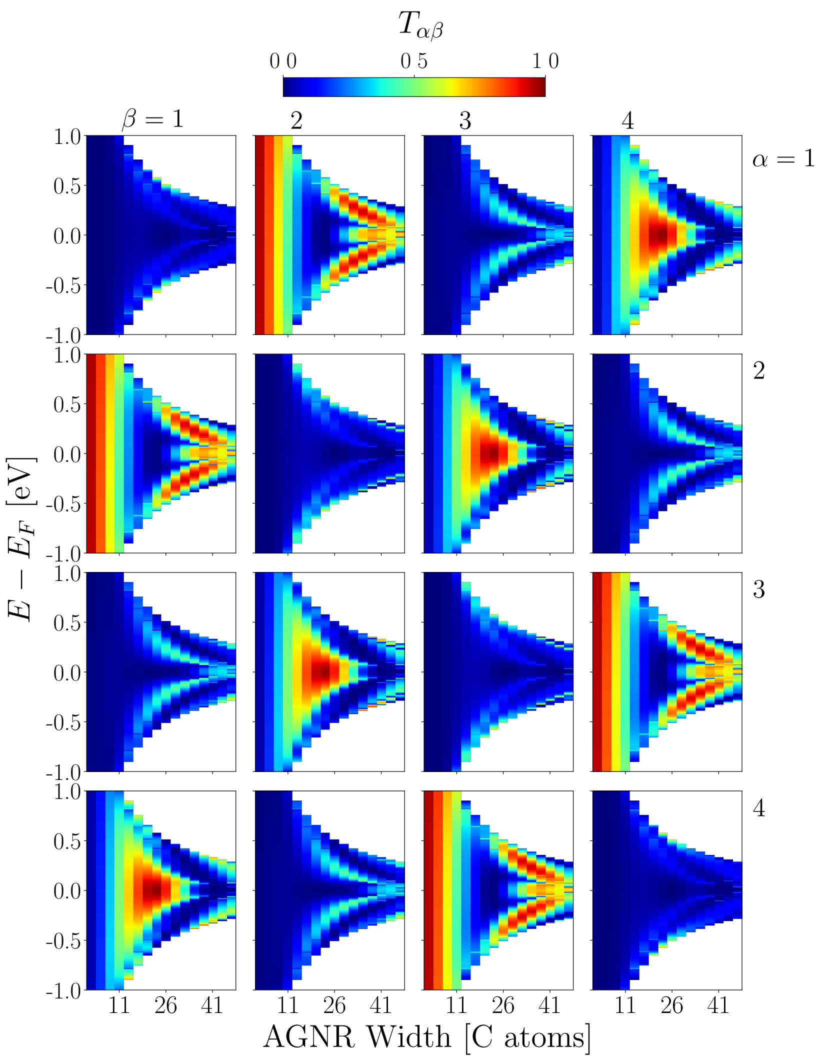


FIG. S5. Transmission probabilities $T_{\alpha\beta}$ for $(3p+2)$-AGNR systems in the the `AA-1` configuration.

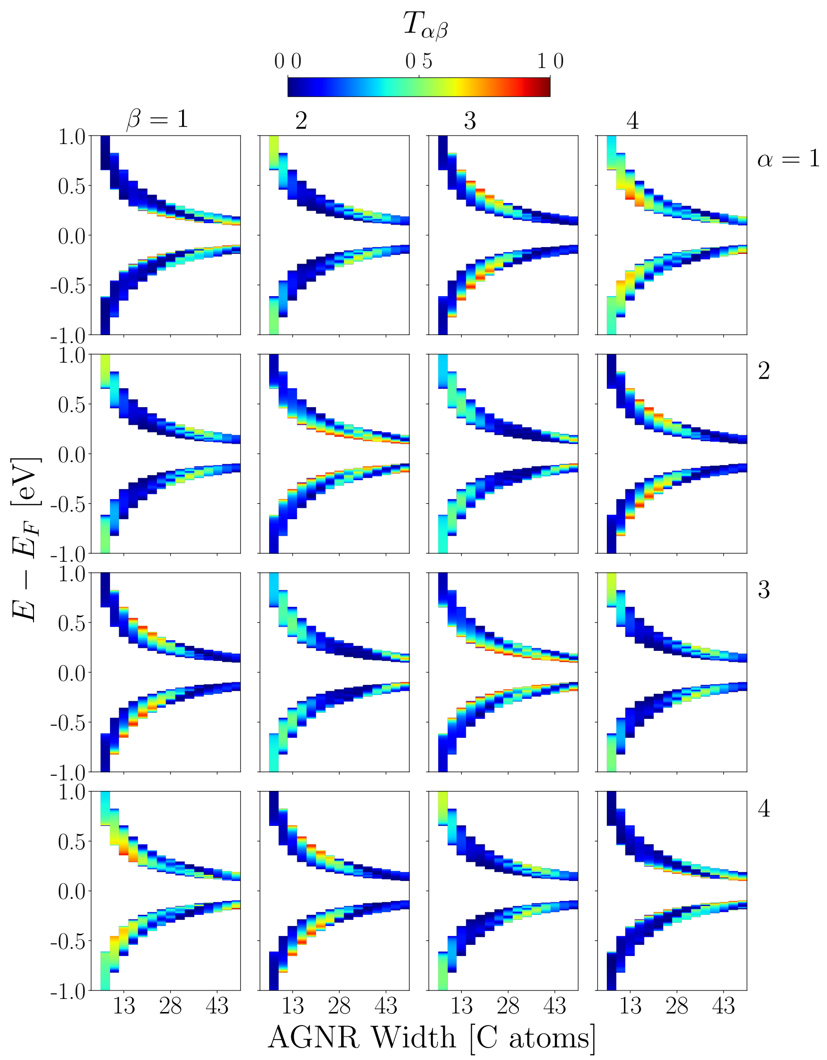


FIG. S6. Transmission probabilities $T_{\alpha\beta}$ for $(3p+1)$-AGNR systems in the the `AA-1` configuration.

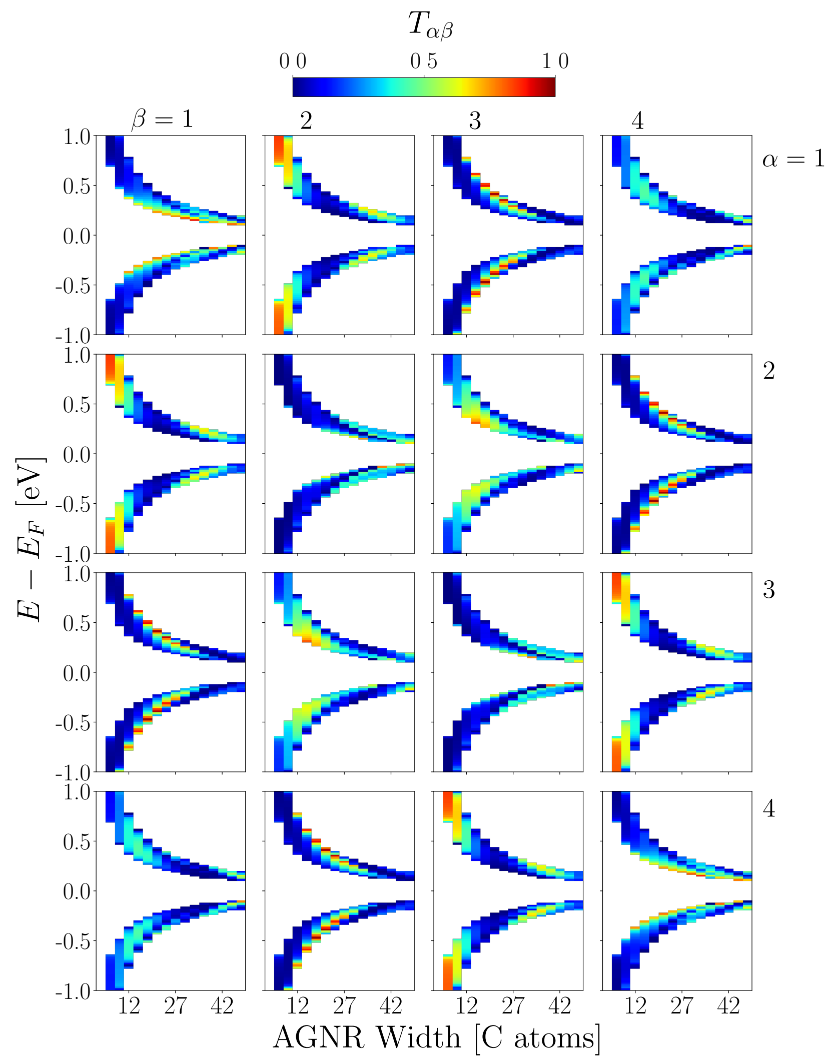


FIG. S7. Transmission probabilities $T_{\alpha\beta}$ for $3p$-AGNR systems in the the `AA-1` configuration.

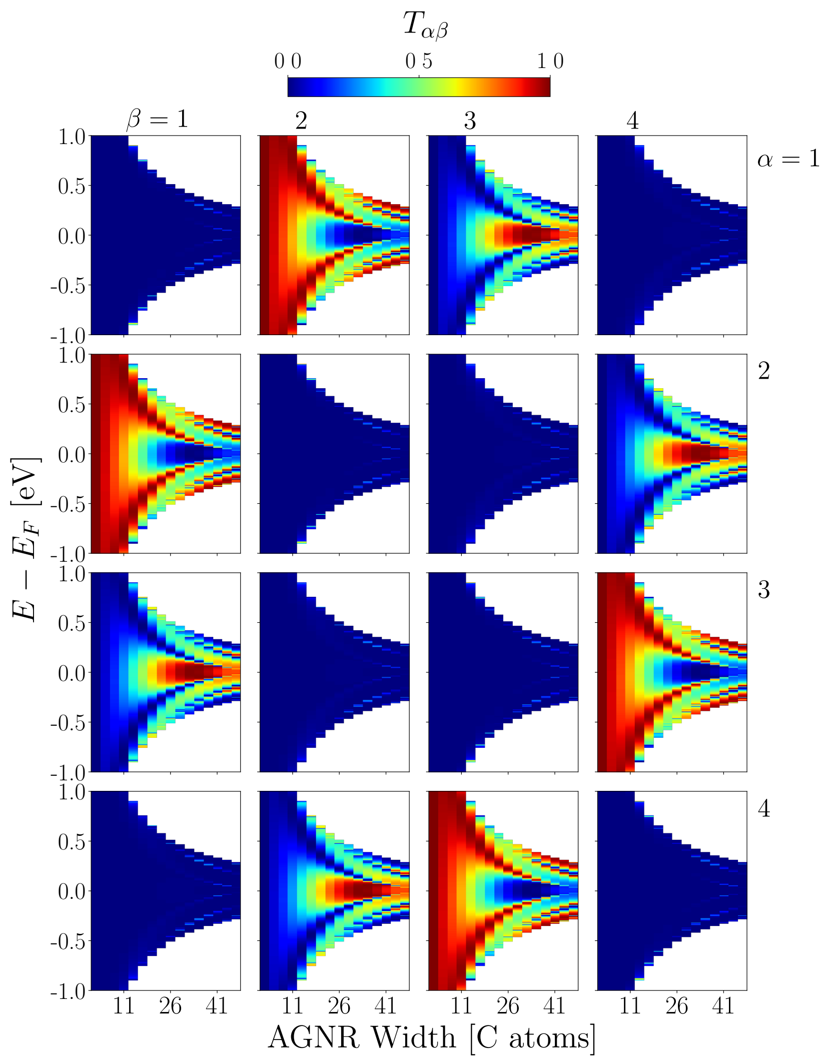


FIG. S8. Transmission probabilities $T_{\alpha\beta}$ for $(3p+2)$-AGNR systems in the the `AA-2` configuration.

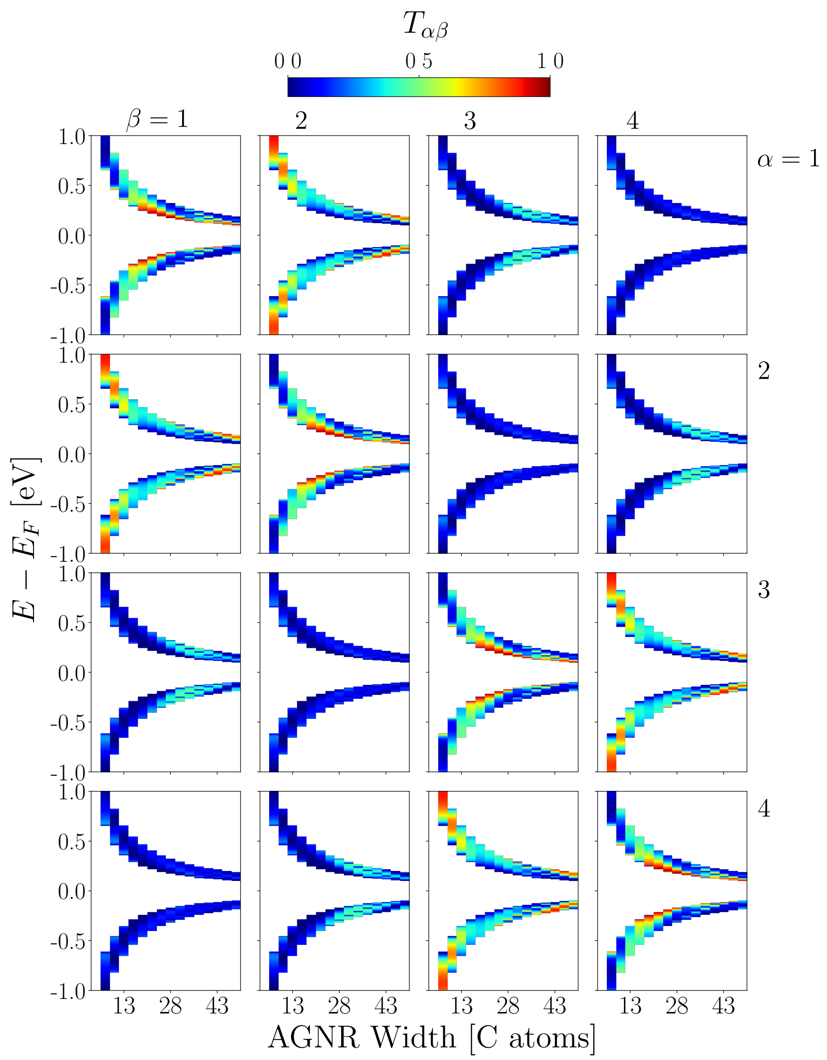


FIG. S9. Transmission probabilities $T_{\alpha\beta}$ for $(3p+1)$-AGNR systems in the the `AA-2` configuration.

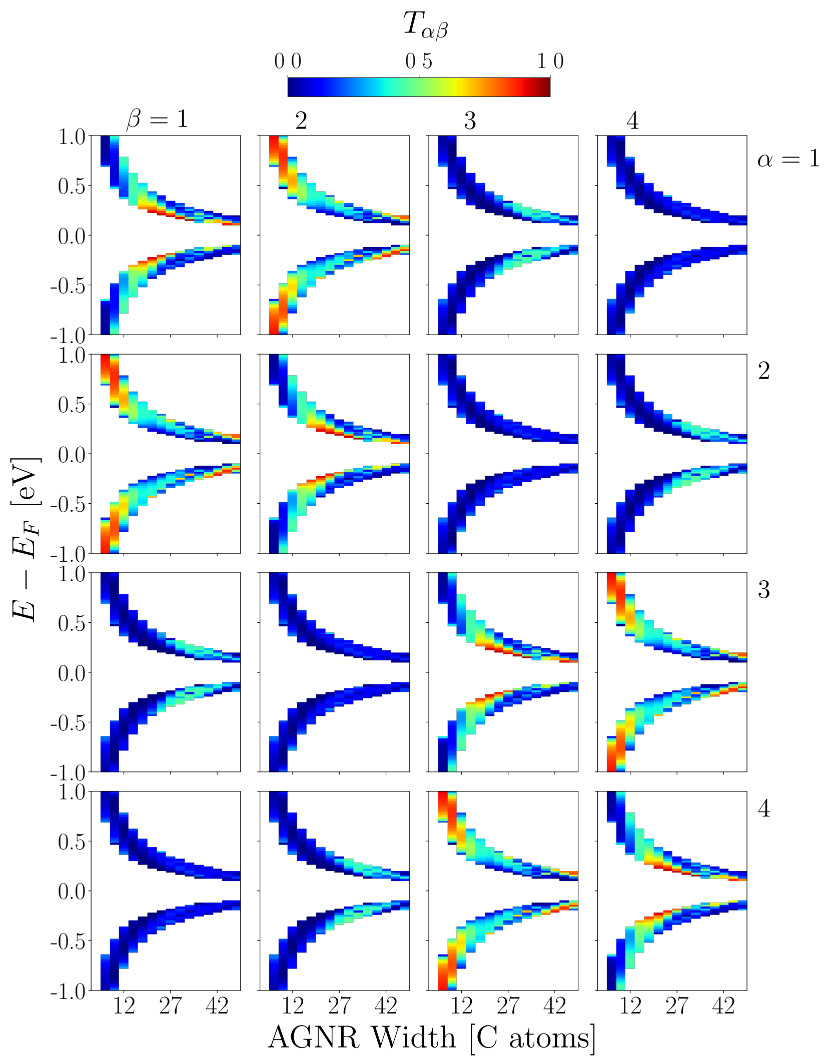


FIG. S10. Transmission probabilities $T_{\alpha\beta}$ for $3p$-AGNR systems in the the `AA-2` configuration.

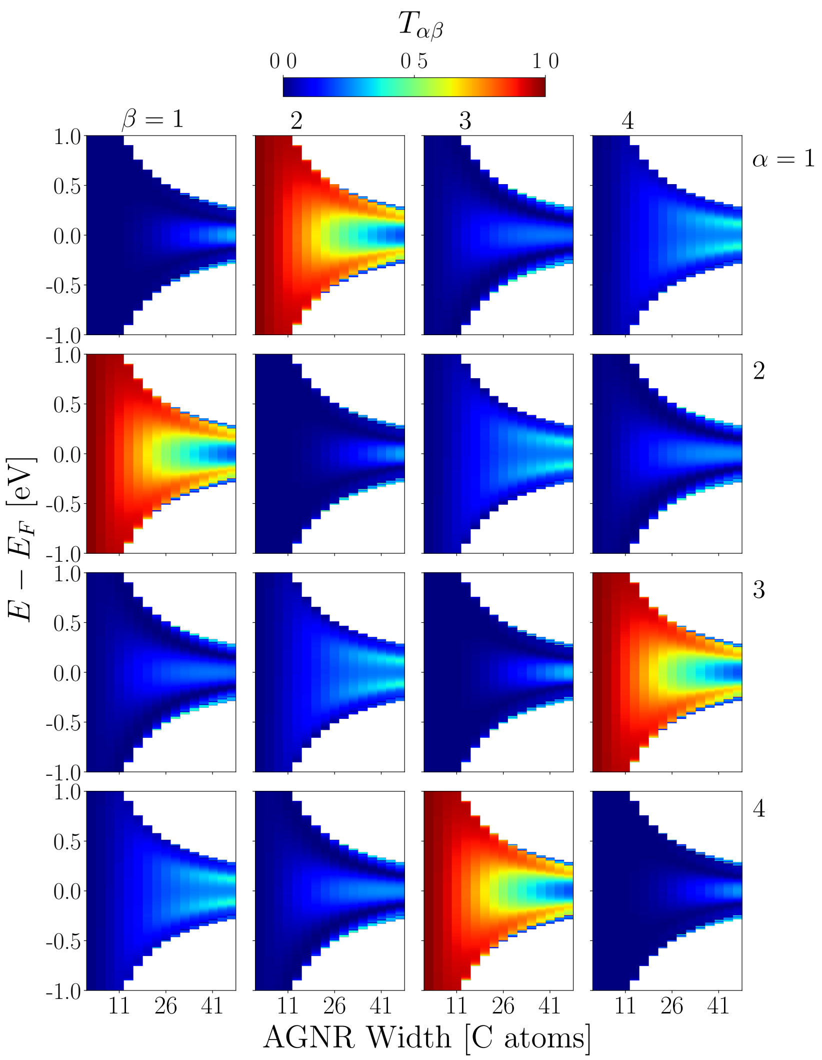


FIG. S11. Transmission probabilities $T_{\alpha\beta}$ for $(3p+2)$-AGNR systems in the the `AB-1` configuration.

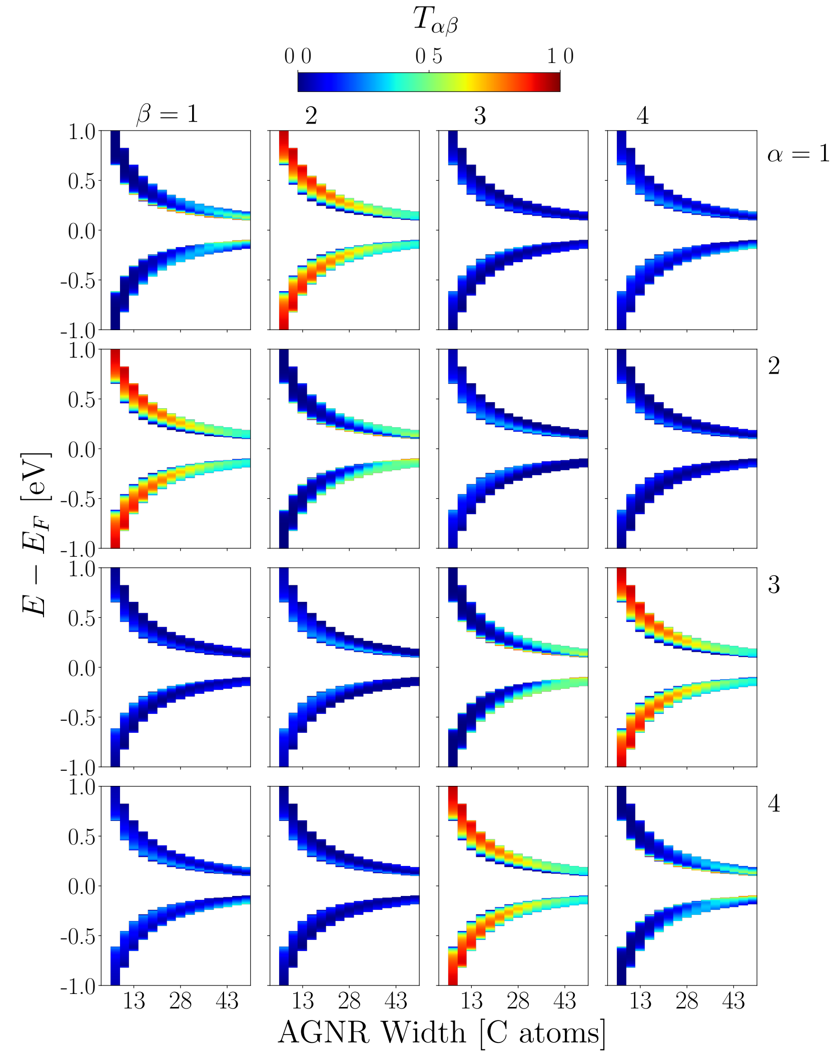


FIG. S12. Transmission probabilities $T_{\alpha\beta}$ for $(3p+1)$-AGNR systems in the the `AB-1` configuration.

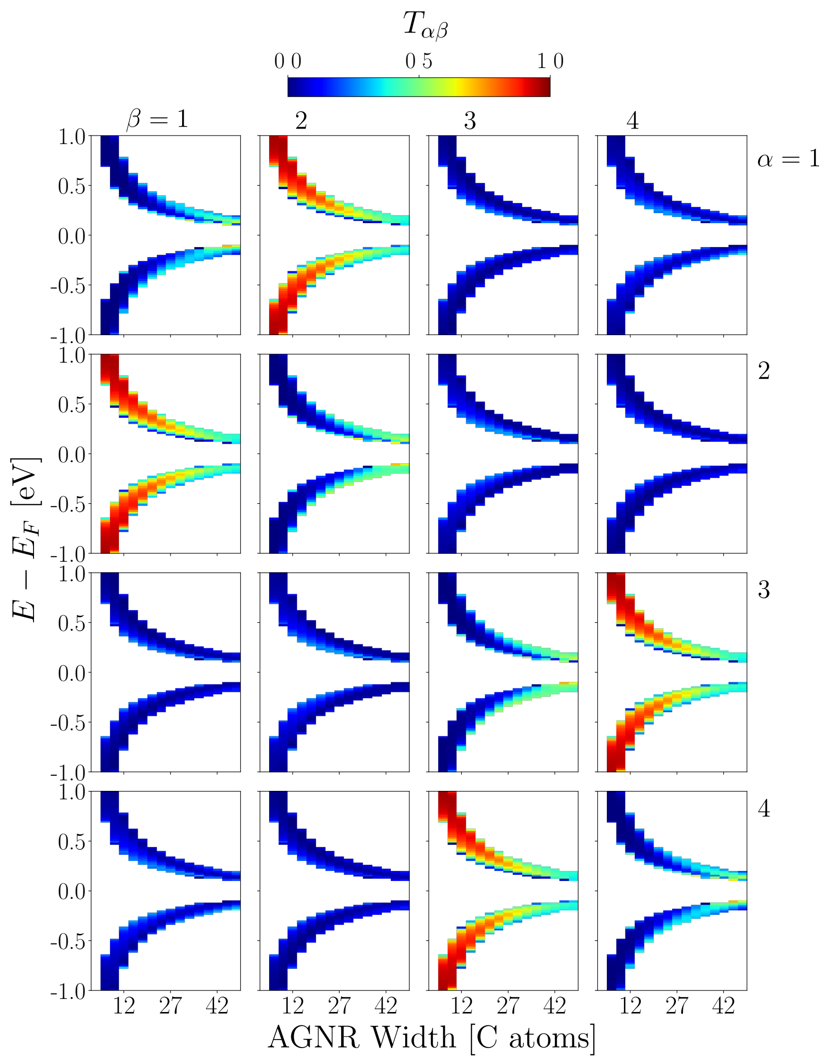


FIG. S13. Transmission probabilities $T_{\alpha\beta}$ for $3p$-AGNR systems in the the `AB-1` configuration.

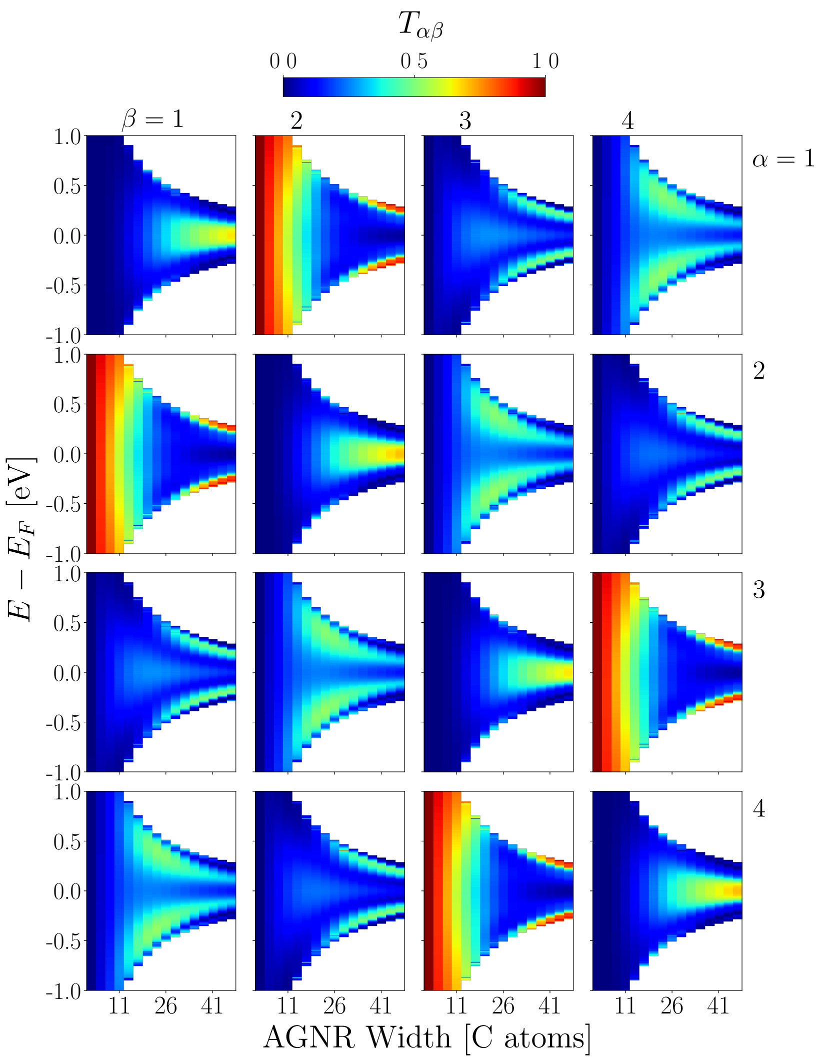


FIG. S14. Transmission probabilities $T_{\alpha\beta}$ for $(3p+2)$-AGNR systems in the the `AB-2` configuration.

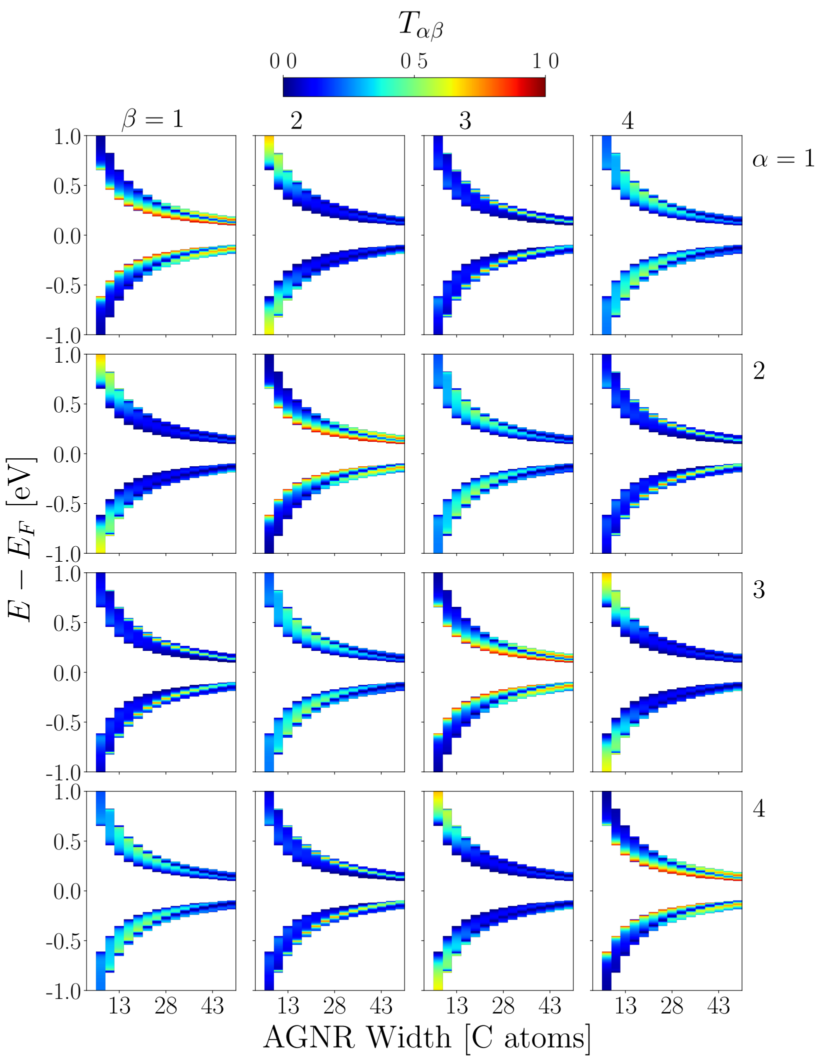


FIG. S15. Transmission probabilities $T_{\alpha\beta}$ for $(3p+1)$-AGNR systems in the the `AB-2` configuration.

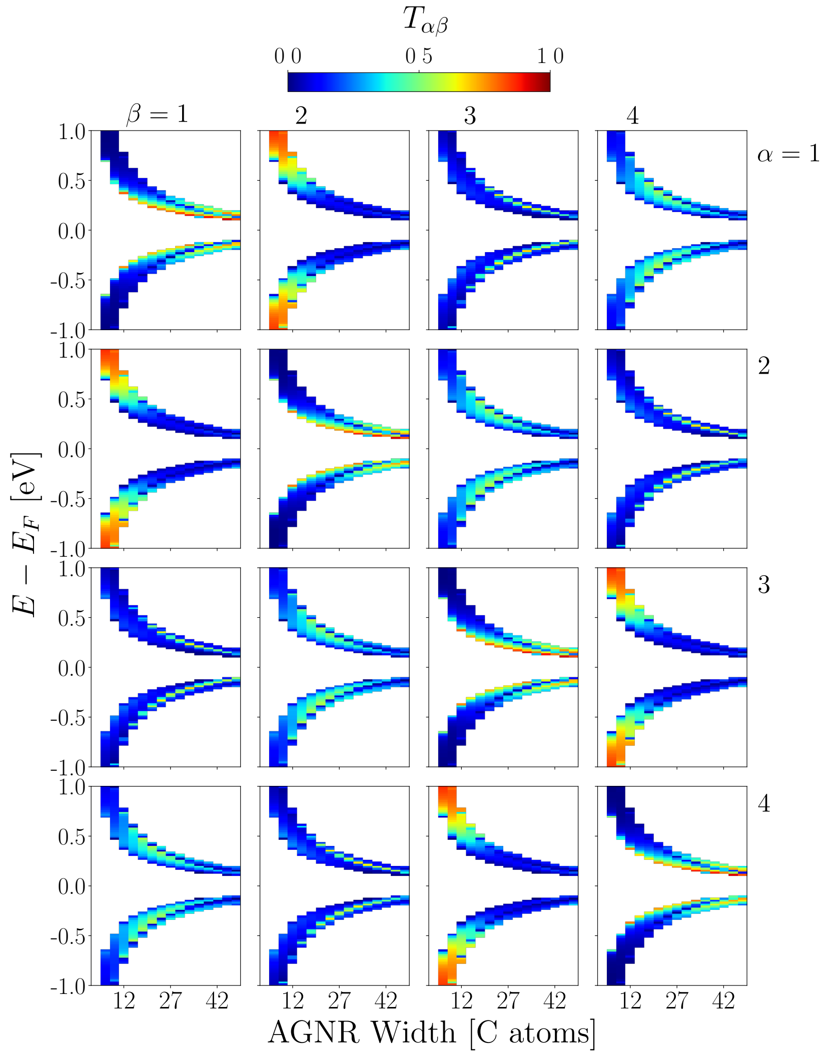


FIG. S16. Transmission probabilities $T_{\alpha\beta}$ for $3p$-AGNR systems in the the `AB-2` configuration.

## S5. BAND STRUCTURE OF MONOLAYER AND BILAYER GNRS

In Fig. S17 we plot the TB band structures for monolayer and bilayer 8-ZGNRs, 16-ZGNRs and 11-AGNRs. The bond length is set to $a = 1.42$ Å, and the separation between the stacked GNRs to $d = 3.34$ Å. Panels (a-c) show the band structure for monolayer and bilayer AA- and AB-stacked 8-ZGNRs, respectively. Panels (d-f) show the band structure for monolayer and bilayer AA- and AB-stacked 16-ZGNRs, respectively. And, panels (g-i) show the band structure for monolayer and bilayer AA- and AB-stacked 11-AGNRs, respectively. We used red color to plot the band structures corresponding to monolayer ZGNR and blue color to plot the band structures of bilayer ZGNRs. All the calculated bands shown in Fig. S17 were obtained using the TB model described in Sec. IIA in the main text.

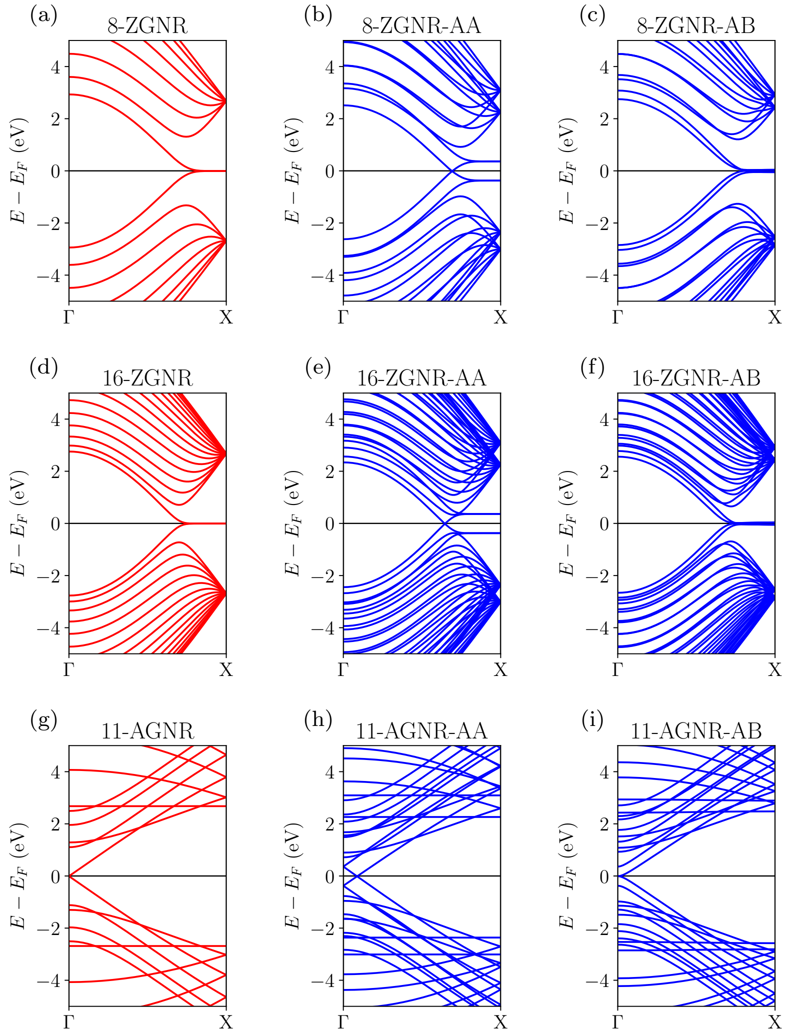


FIG. S17. Band structures of monolayer and bilayer-GNRs. Band structure along the path Γ–X for (a) monolayer and, (b) AA- and (c) AB-stacked 8-ZGNRs, (d) monolayer and bilayer (e) AA-stacked and (f) AB-stacked 16-ZGNRs, and (g) monolayer and bilayer (h) AA-stacked and (i) AB-stacked 11-AGNRs. All the calculated bands were obtained with the TB model described in Sec. IIA in the main text.

## S6. TRANSMISSION PEAKS AS A FUNCTION OF THE RIBBON WIDTH

In this section we show the reflection ($R_1$) and transmission ($T_{12}, T_{13}, T_{14}$) probabilities as a function of the ribbon widths for `AA`-stacked ZGNRs and `AA-2`-stacked $(3p+2)$-AGNRs. In Fig. S18 we plot these probabilities for ZGNRs of $W \in [8, 16]$ C atoms (panel (a)), and for AGNRs of $W \in [8, 32]$ C atoms (panel (b)) as a function of the incoming electron energy.

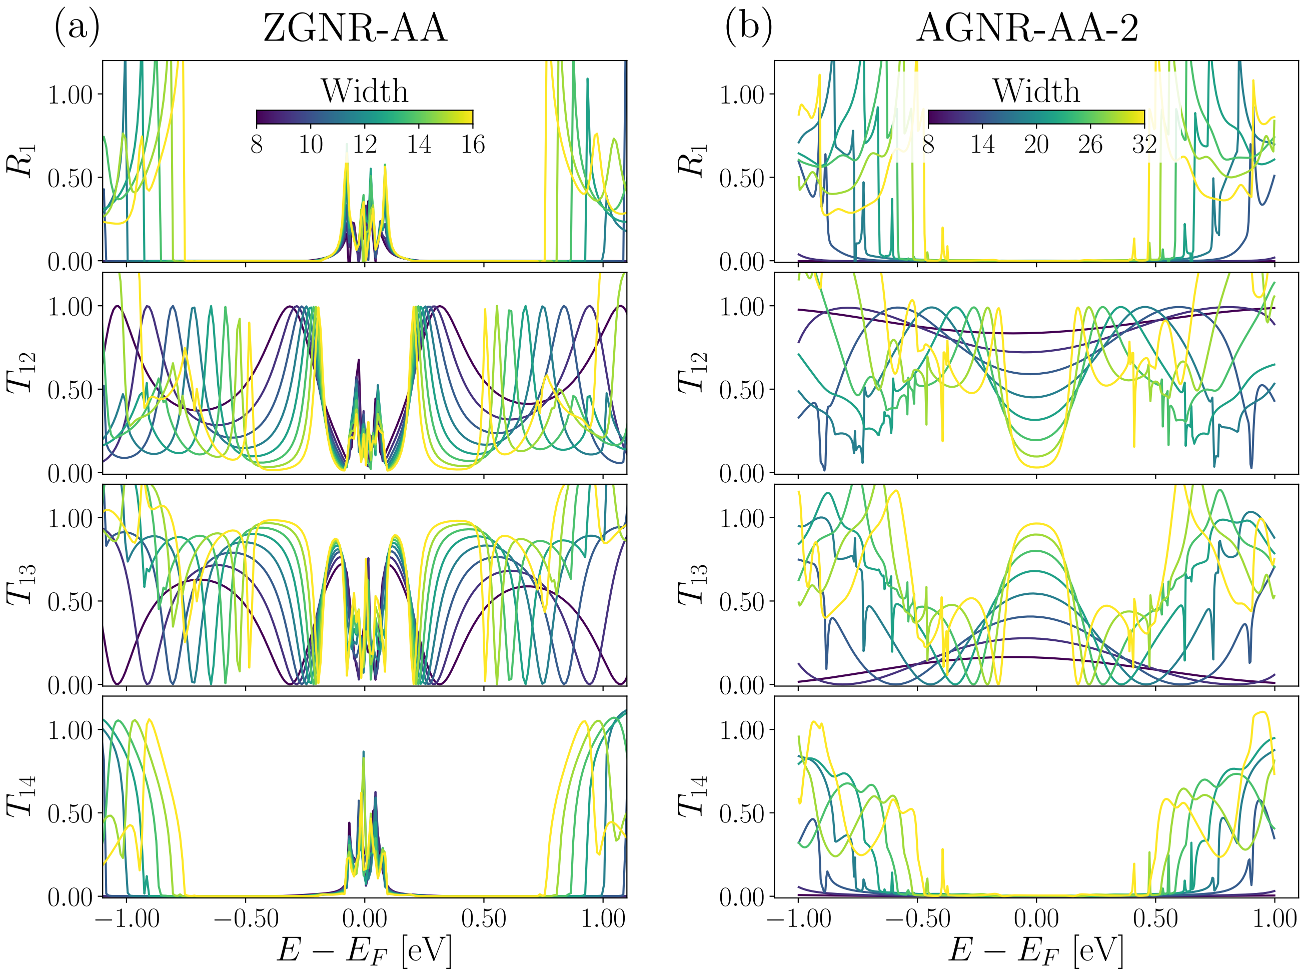


FIG. S18. Transmission and reflection probabilities for ribbons of different widths. Reflection $R_1$ and transmission $T_{12}, T_{13}, T_{14}$ as a function of the incoming electron energy $E - E_F$ obtained for many GNRs' widths (color lines) for (a) two crossed ZGNRs in the `AA` configuration, and (b) two crossed AGNRs (of width $W = 3p + 2$) in the `AA-2` configuration.

## S7. ROBUSTNESS OF TRANSPORT PROPERTIES FOR AA-STACKED ZGNRS

In the main text we presented and discussed the variability of the transport properties of `AB`-stacked 8-ZGNR devices in Sec. III.E against some perturbations. Here we complement those results with the same calculations performed on `AA`-stacked devices (Figs. S19-S23). All graphs are compared to the reference case (`AA`-stacked 8-ZGNRs), which is plotted in black lines.

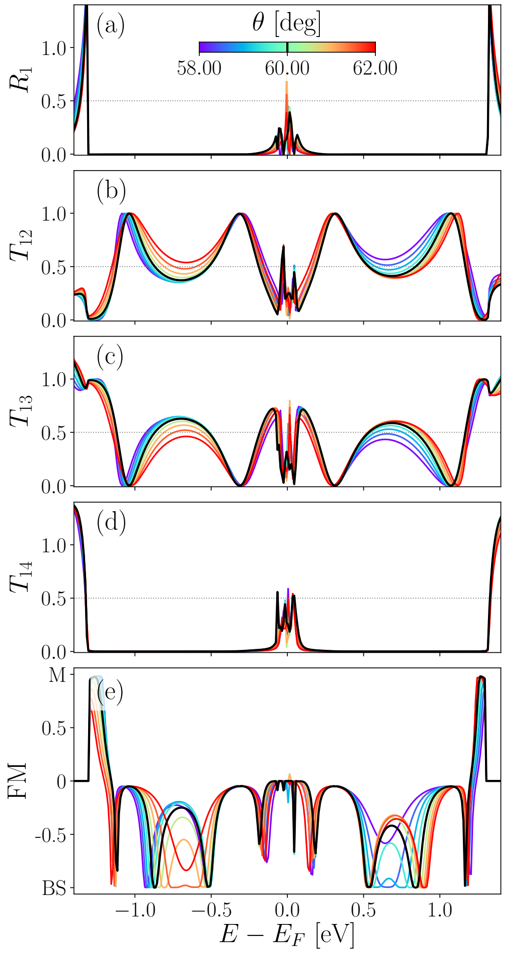


FIG. S19. Variation with respect to the rotation angle between two `AA`-stacked 8-ZGNRs. Reflection and transmission probabilities, (a) $R_1$ (b) $T_{12}$, (c) $T_{13}$ and (d) $T_{14}$, and (e) figure of merit (FM) as a function of the incoming electron energy $E - E_F$, obtained for different relative angles ($\theta$) between the ribbons (color lines).

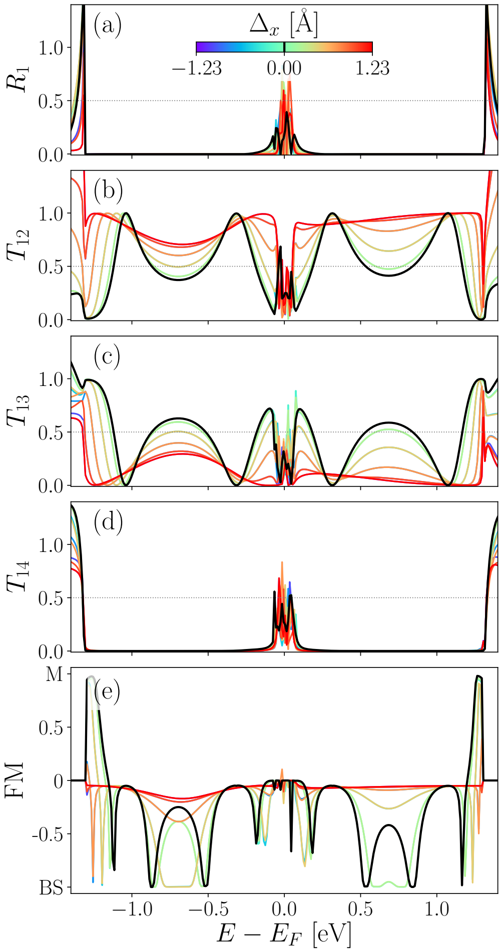


FIG. S20. Variation with respect to the lateral displacement between two AA-stacked 8-ZGNRs. Reflection and transmission probabilities, (a) $R_1$ (b) $T_{12}$, (c) $T_{13}$ and (d) $T_{14}$, and (e) figure of merit (FM) as a function of the incoming electron energy $E - E_F$, obtained for different translation distances along the $x$-axis ($\Delta_x$) of the on-top ribbon (color lines).

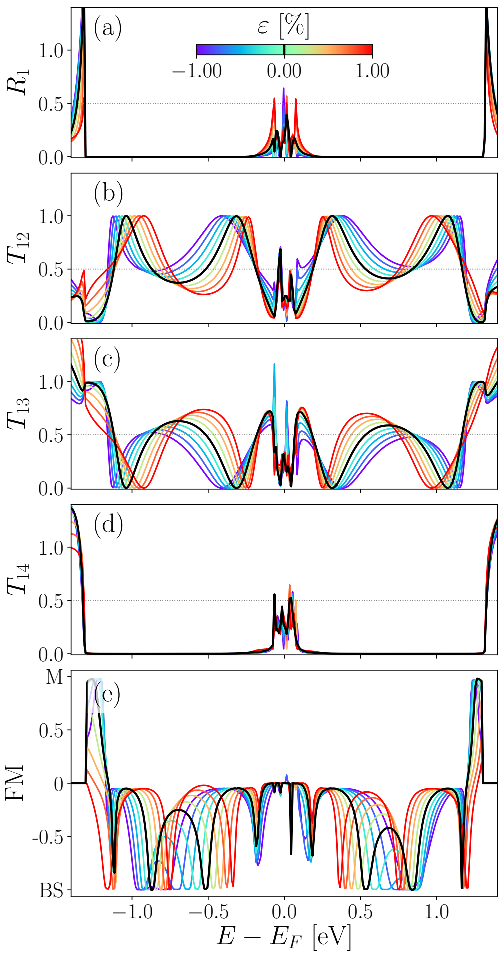


FIG. S21. Variation with respect to the applied uniaxial strain along the periodic direction of each GNR for the two `AA`-stacked 8-ZGNRs. Reflection and transmission probabilities, (a) $R_1$ (b) $T_{12}$, (c) $T_{13}$ and (d) $T_{14}$, and (e) figure of merit (FM) as a function of the incoming electron energy $E - E_F$, obtained for different uniaxial strain $\varepsilon$ applied to both GNRs along the non-confined direction (color lines).

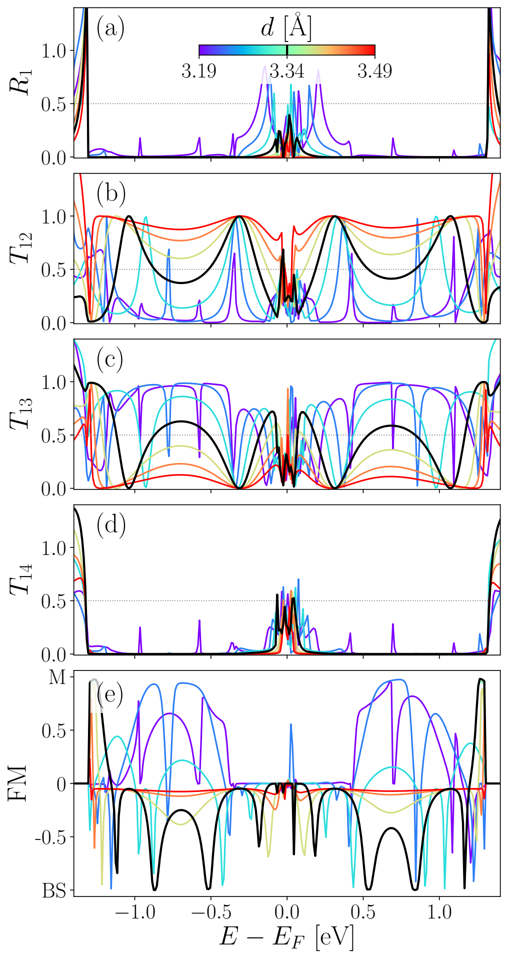


FIG. S22. Variation with respect to the *inter*-GNR separation $d$ between the two AA-stacked 8-ZGNRs. Reflection and transmission probabilities, (a) $R_1$ (b) $T_{12}$, (c) $T_{13}$ and (d) $T_{14}$, and (e) figure of merit (FM) as a function of the incoming electron energy $E - E_F$, obtained for different separations ($d$) between the ribbons (color lines).

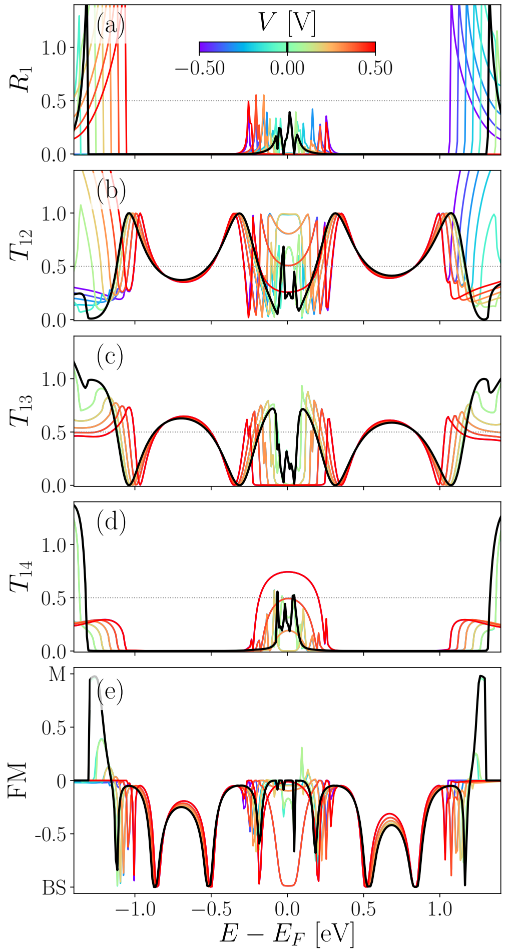


FIG. S23. Variation with respect to the applied voltage between the two AA-stacked 8-ZGNRs. Reflection and transmission probabilities, (a) $R_1$ (b) $T_{12}$, (c) $T_{13}$ and (d) $T_{14}$, and (e) figure of merit (FM) as a function of the incoming electron energy $E - E_F$, obtained for different applied voltages ($V$) between the ribbons (color lines).

[1] T. N. Todorov, J. Phys: Condens. Matter **14**, 3049 (2002).
[2] N. Papior, N. Lorente, T. Frederiksen, A. García, and M. Brandbyge, Comp. Phys. Commun. **212**, 8 (2017).
[3] Y.-W. Son, M. L. Cohen, and S. G. Louie, Nature **444**, 347 (2006).
[4] Y.-W. Son, M. L. Cohen, and S. G. Louie, Phys. Rev. Lett. **97**, 216803 (2006).
[5] L. Yang, C.-H. Park, Y.-W. Son, M. L. Cohen, and S. G. Louie, Phys. Rev. Lett. **99**, 186801 (2007).
[6] T. Wassmann, A. P. Seitsonen, A. M. Saitta, M. Lazzeri, and F. Mauri, Phys. Rev. Lett. **101**, 096402 (2008).
